# Supplementary material for: Continuous body 3-D reconstruction of limbless animals
Source: arXiv:2103.05198 ancillary file (2025-10-11)
Supplement: Supplementary file 1 [file Snake_modeling_arXiv_SM.pdf]

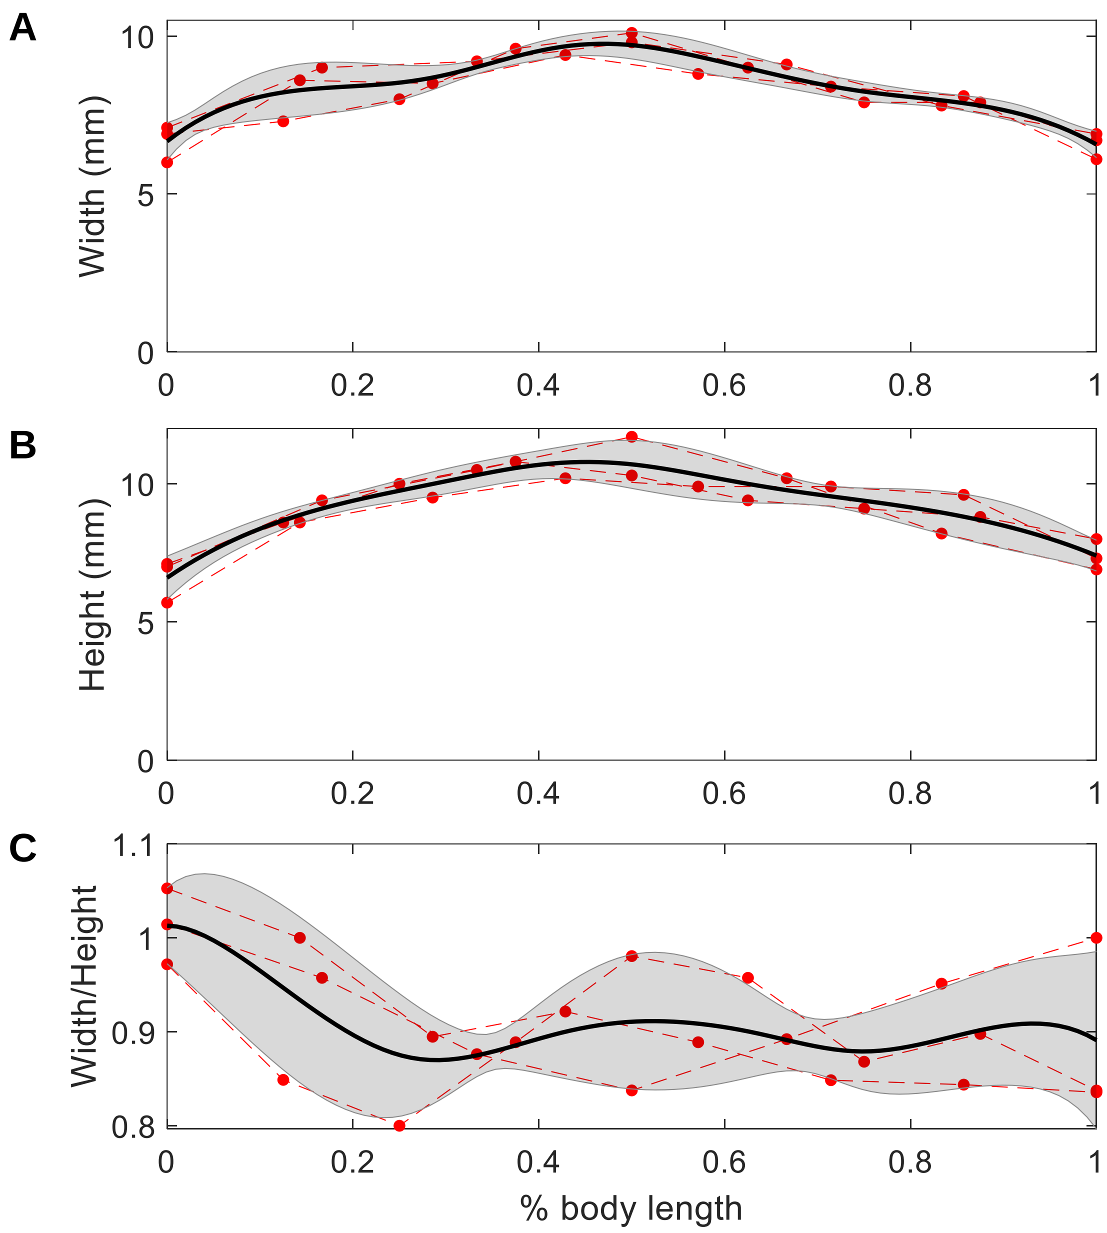


**Fig. S1. Kingsnake's body width, height, and tapering.** (A) Body width, (B) body height, and (C) aspect ratio (width divided by height) measured at different locations along the body. Red markers show measurement points for each individual. Black curves and shaded area show mean ± s.d. Because we could not measure at the exact same body locations for each snake, we linearly interpolated measurements along the body.

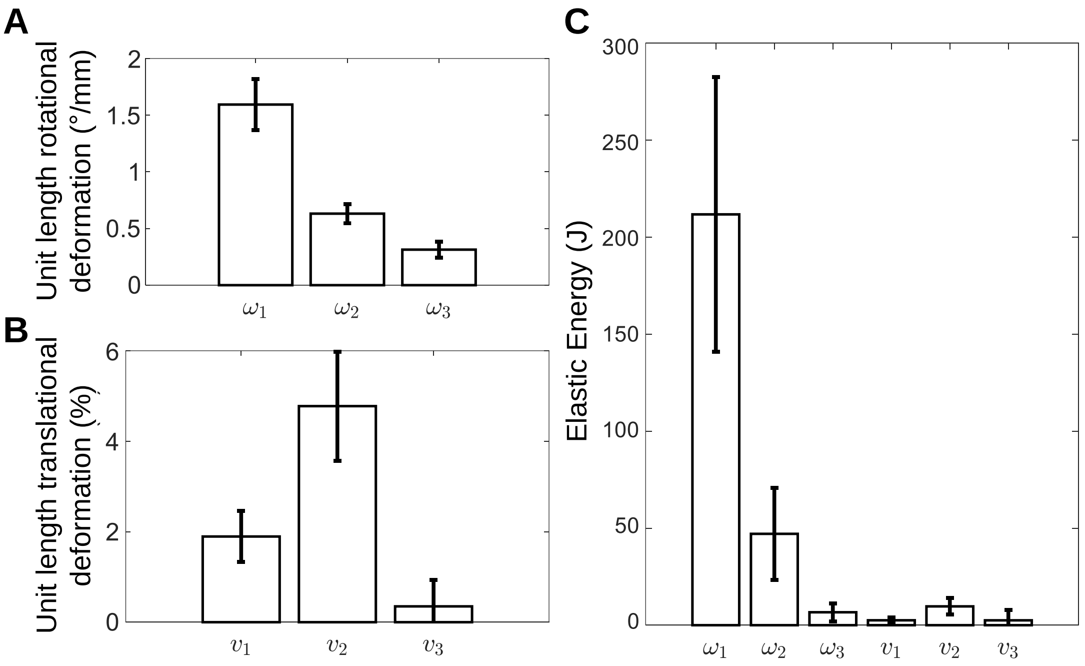


**Fig. S2. Comparison of the amount of different types of elastic rod deformation.** (A) Unit length rotational deformation, including $\omega_1$, $\omega_2$ (lateral and dorsoventral bending), and $\omega_3$ (twisting). (B) Unit length translational deformation, including $v_1$, $v_2$ (lateral and dorsoventral shearing), and $v_3$ (extension and compression). (B) Contributions to elastic energy of all six types of elastic rod deformation.

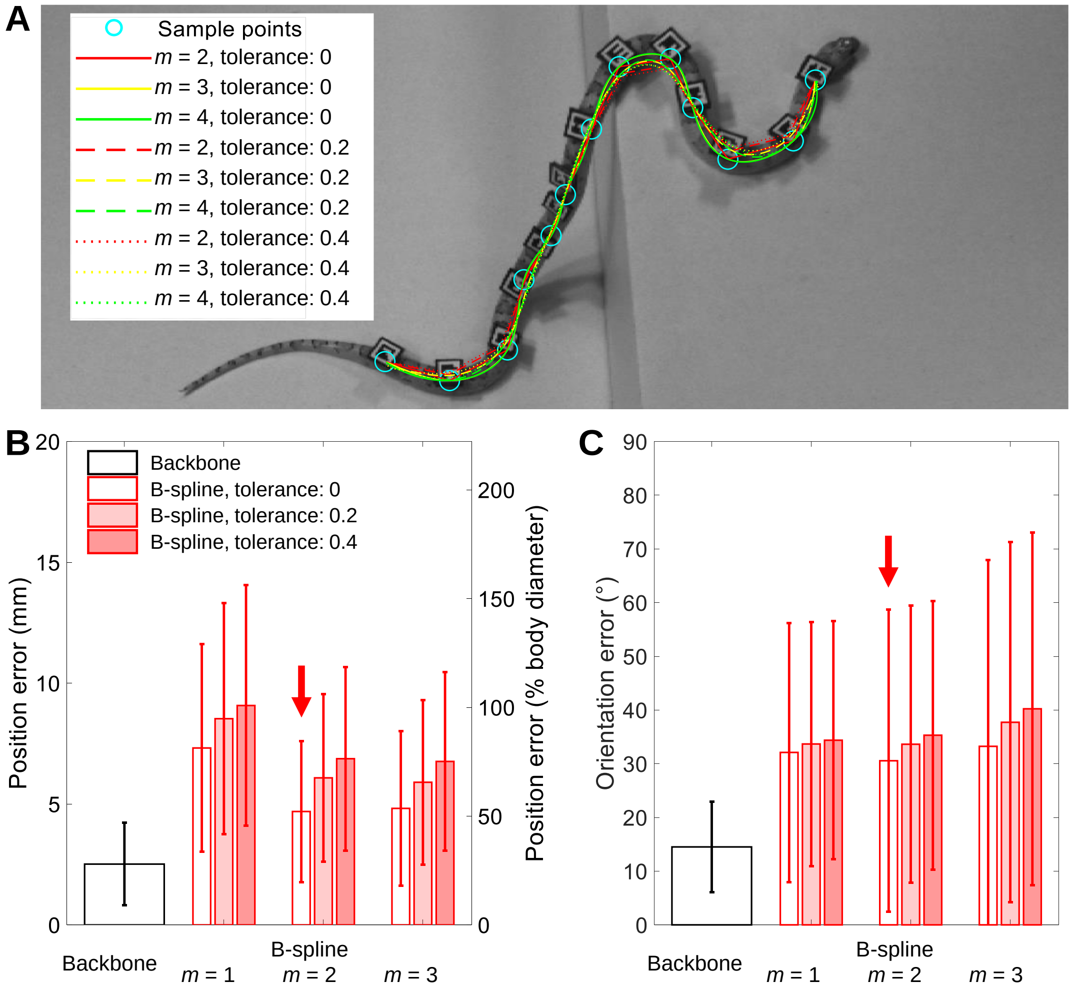


**Fig. S3. Comparison of our method with B-spline method using different parameters.** (A) A representative snapshot of interpolation results using B-spline with different parameters. (B) Position error. (C) Orientation error. $2m$–1 is the degree of B-spline basis function, tolerance multiplied by body length is the tolerance parameter *tol* for interpolating $\boldsymbol{p}$ or $\boldsymbol{r}_1$, $\boldsymbol{r}_2$, $\boldsymbol{r}_3$. Arrow indicates result shown in Fig. 3 in main text using cubic ($m$ = 2) B-spline with zero tolerance most commonly used in animal locomotion literature (Sharpe et al., 2015; Fontaine et al., 2008; Yeaton et al., 2020).
